# Supplementary material for: $Z_2$ flux binding to higher-spin impurities in the Kitaev spin liquid
Source: arXiv:2409.02190 source file (2025-02-01)
Supplement: Supplementary file 1 [file suppl.pdf]

# Supplementary Information for "$Z_2$ flux binding to higher-spin impurities in the Kitaev spin liquid"

Masahiro O. Takahashi[1], Wen-Han Kao[2], Satoshi Fujimoto[1], and Natalia B. Perkins[2]

[1]Department of Materials Engineering Science, Osaka University, Toyonaka 560-8531, Japan

[2]School of Physics and Astronomy, University of Minnesota, Minneapolis, Minnesota 55455, USA

January 14, 2025

We have employed the density matrix renormalization group (DMRG) method to evaluate the ground state flux sector of the Kitaev honeycomb model with magnetic impurities across various finite-size clusters. In most part of this supplementary information, we discuss the impurity position dependence of the flux-sector transition [as shown in Supplementary Figure 1] and the results from two impurities on the cluster [as shown in Supplementary Figure 4]. In the final subsection, we also comment on flux-sector transitions observed in other finite-size clusters.

## Supplementary Note 1: 48-site cluster on the cylinder geometry

The 48-site cluster used in the main text is shown in Supplementary Figure 1**a**. For the $L_\theta$ ($L$) direction, we applied periodic (open) boundary conditions, respectively, resulting in a cylindrical geometry. This cylindrical cluster always satisfies the bound-flux sector at $g/J = 0$ even for a single impurity case. Note that this cluster has an inversion symmetric point located at the midpoint between sites 22 and 27 and discrete translational symmetry in the $L_\theta$ direction.

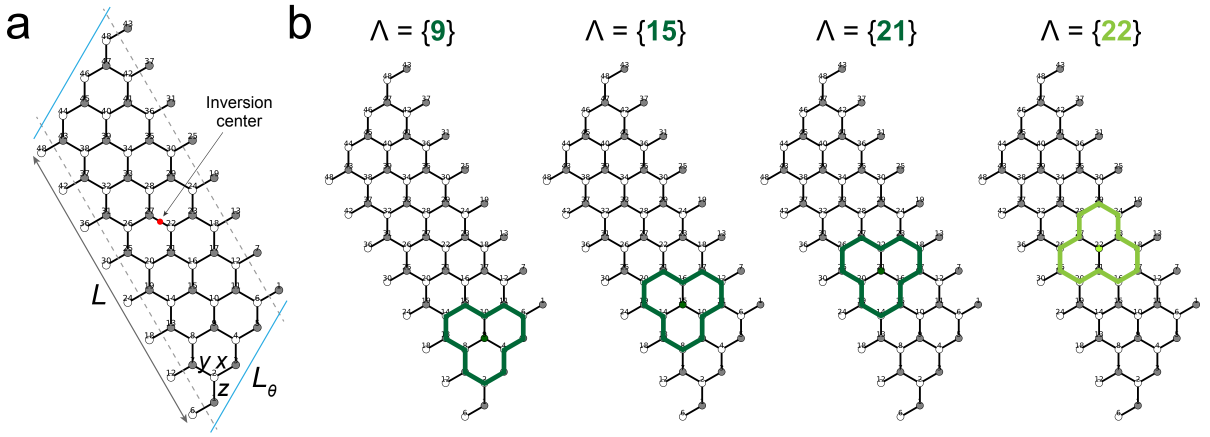


Supplementary Figure 1. **a** The 48-site cluster used in the DMRG calculations. **b** Different positions of the single-impurity site in the cluster. Dark (light) green color on the site numbers denote the A (B) sublattice.

In Supplementary Table 1, we summarize flux sector transitions depending on the impurity position and the spin size of the impurity site. We denote the first transition point from the bound-flux sector to the zero-flux sector as $g_1$, and the second transition point from the zero-flux sector to the reentrant bound-flux sector as $g_2$. The $\Lambda = \{21\}$ case is selected as a typical example discussed in the main text. The qualitative trend of the transition points shown in Supplementary Table 1 will be discussed in depth in the following subsections.

Supplementary Table 1. Flux sector transitions depending on the impurity position and the spin size of the impurity. **B** (**Z**) represents the bound-flux (zero-flux) sector, respectively.

| | | $S_{\text{imp}} = 1/2$ | $S_{\text{imp}} = 1$ | $S_{\text{imp}} = 3/2$ |
|---|---|---|---|---|
| $\Lambda = \{9\}$ | Flux sector | **B - Z** | **B - Z** | **B** |
| | $g_1$ | 0.82 | 0.88 | - |
| | $g_2$ | - | - | - |
| $\Lambda = \{15\}$ | Flux sector | **B - Z** | **B - Z** | **B - Z - B** |
| | $g_1$ | 0.44 | 0.38 | 0.48 |
| | $g_2$ | - | - | 0.72 |
| $\Lambda = \{21\}$ | Flux sector | **B - Z** | **B - Z** | **B - Z - B** |
| | $g_1$ | 0.25 | 0.20 | 0.15 |
| | $g_2$ | - | - | 0.40 |
| $\Lambda = \{22\}$ | Flux sector | **B - Z** | **B - Z - B** | **B - Z - B** |
| | $g_1$ | 0.12 | 0.08 | 0.08 |
| | $g_2$ | - | 0.74 | 0.16 |

## Supplementary Note 2: Flux gap in the cylinder geometry

First, we consider the single-vacancy case and examine the position dependence of the flux gap, which is defined as the energy difference between the bound-flux and the zero-flux sectors, $\Delta E = E_{\text{bound}} - E_{\text{zero}}$. In Supplementary Figure 2**a**, the ground state energy (GSE) of both sectors and their energy difference ($\Delta E$) at $g = 0$ are calculated by the exact diagonalization in the usual Majorana representation [1]. The GSE of the zero-flux sector exhibits little position dependence from the edge ($\Lambda = \{9\}$) to the bulk ($\Lambda = \{21\}$). In contrast, the GSE of the bound-flux sector monotonically increases as the impurity moves away from the edge, resulting in a shrink of the flux gap. The position dependence on GSE of the bound-flux sector is also confirmed in the DMRG calculation.

It is worth comparing the above trend to the pure Kitaev model with flux proliferation. In the pure Kitaev model, the ground-state sector is always zero-flux, and the single-flux gap diminishes as the flux moves *closer* to the edge [2]. Therefore, thermal fluxes proliferate more easily on the edge instead of in the bulk. On the other hand, for the system with a quasivacancy (that is, a $S_{\text{imp}} = 1/2$ impurity), the bound-flux sector is more stable when it gets closer to the edge. This qualitative behavior is valid for small but nonzero $g$ as shown in Supplementary Figure 2**b**. Nevertheless, one should also notice that larger values of $g$ may cause instability, leading to the $g_1$ transition from the bound-flux to the zero-flux sector, which will be discussed next.

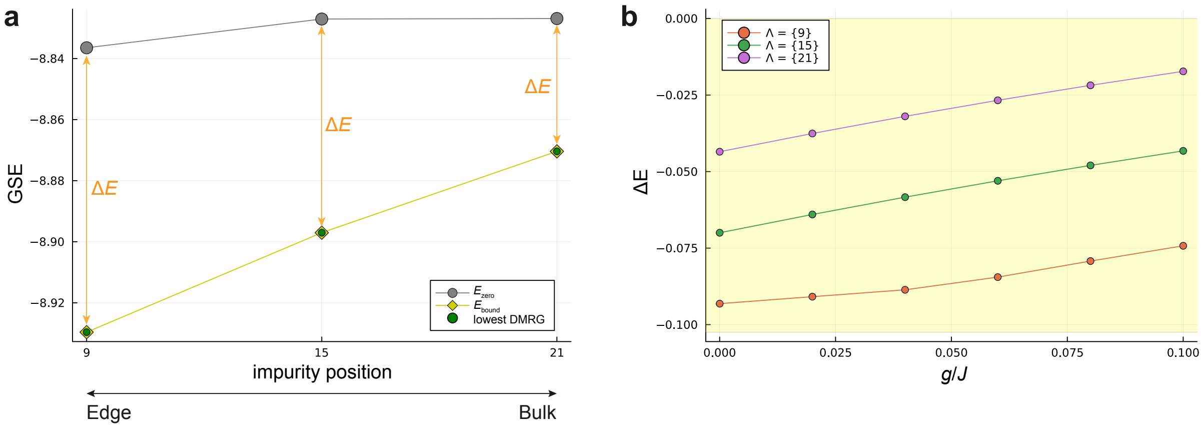


Supplementary Figure 2. **a** Ground state energies at the zero-flux and the bound-flux sectors. The energy difference corresponds to the single flux gap, which depends on the impurity position. **b** Impurity position dependence on the energy difference $\Delta E$ at small $g/J$ regime calculated in the Kitaev spin liquid with a quasivacancy ($S_{\text{imp}} = 1/2$).

## Supplementary Note 3: Impurity position dependence on transitions

Here we discuss the impurity-position dependence of the flux-sector transitions in Supplementary Table 1. In the small-$g$ region as shown in Supplementary Figure 2(b), the bound-flux sector becomes more stable as the impurity site approaches the edge, regardless of the impurity spin size. This can be readily verified by examining the existence and position of $g_1$ in the same column of Supplementary Table 1. This behavior can be explained by the impurity-position dependence of the energy difference $\Delta E$.

Furthermore, for $S_{\mathrm{imp}} = 3/2$, the emergence of the reentrant bound-flux sector at $g \geq g_2$ also depends on the impurity position. We observe that the second transition point, $g_2$, decreases as the impurity is positioned farther from the edge. In addition, we do not observe the third transition from the reentrant bound-flux sector to the "reentrant zero-flux sector" for any impurity position within $0 \leq g/J \leq 10.0$ regime. This supports the robustness of the bound-flux sector in the system with $S_{\mathrm{imp}} = 3/2$ impurities.

In the large-$g$ limit, while the ground state for $S_{\mathrm{imp}} = 3/2$ is in the bound-flux sector for all cases, the ground state for $S_{\mathrm{imp}} = 1$ exhibits some position dependence. This qualitative difference can be seen by comparing two cases, $\Lambda = \{21\}$ and $\Lambda = \{22\}$. From the case of $\Lambda = \{21\}$ to $\Lambda = \{22\}$ for $S_{\mathrm{imp}} = 1$, the value of $g_1$ decreases and the second transition emerges. This property may be understood through a phenomenological description based on the effective coupling model discussed in the main text, where the position dependence of the impurity site affects all parameters $A_1, B_{1,2}$, and $C_{1,2}$ in Eq. (18) of the main text. This results in differences such as curvature and a constant shift in the energy of the quadratic curve between two cases, suggesting the possibility of a reentrant bound-flux sector in a specific impurity position case within the validity of the parameter regime $\Delta \ll 1$. Thus, we conclude that $\Delta E$ in the $S_{\mathrm{imp}} = 1$ impurity case is somewhat marginal and sensitive to the impurity position, making it a subtle system that warrants further investigation. As discussed in the main text, the subtlety of the $S_{\mathrm{imp}} = 1$ is not only rooted in the trend of the impurity spin size, but also in the absence of conserved values for internal plaquette operators. In Supplementary Figure 3**b**, we present the flux-sector phase diagram for $S_{\mathrm{imp}} = 1$ with $\Lambda = \{21\}$ and $\Lambda = \{22\}$. Even though the $\Lambda = \{22\}$ case reveals a reentrant bound-flux sector at large $g$, it is quite fragile against the external magnetic field, compared with the $S_{\mathrm{imp}} = 3/2$ phase diagram in the main text. This implies that the $S_{\mathrm{imp}} = 1$ system may not be an ideal system for stabilizing an Ising anyon around the defect, compared with other proposals such as vacancies [3], Kondo impurities [4, 5], and spin-3/2 magnetic impurities.

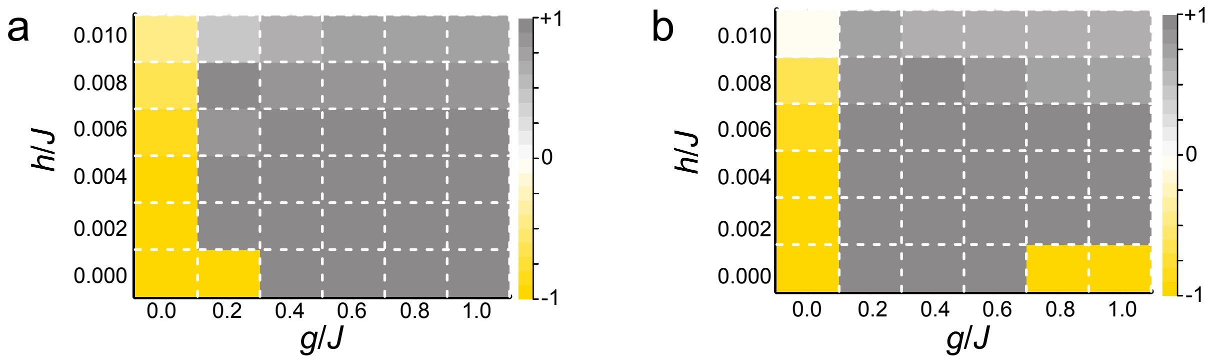


Supplementary Figure 3. Phase diagrams of one spin-1 impurity case calculated in the 48-site cylinder. The magnetic field $\mathbf{h}$ is along [111] direction. **a** The impurity is located at the site $\Lambda = \{21\}$. This figure is the same as Fig.2**b** in the main text. **b** The impurity is located at the site $\Lambda = \{22\}$. The reentrant bound-flux sector emerges for large $g$, but it is fragile against the magnetic field. The site positions are shown in Fig. Supplementary Figure 1.

## Supplementary Note 4: 48-site cluster with two impurities

Here, we present the numerical results on the ground-state flux sectors for two impurities. For demonstrating the position dependence, we choose four different impurity configurations on the 48-site cluster, as shown in Supplementary Figure 4**a-d**. Since there are two impurity plaquettes, we calculate the sum of the two triple-plaquette operators $\sum_{\lambda=\mathrm{A,B}} W_{I\lambda}$. In Supplementary Figure 4**e-g**, we summarize the ground-state flux sector as a function of coupling strength $g$.

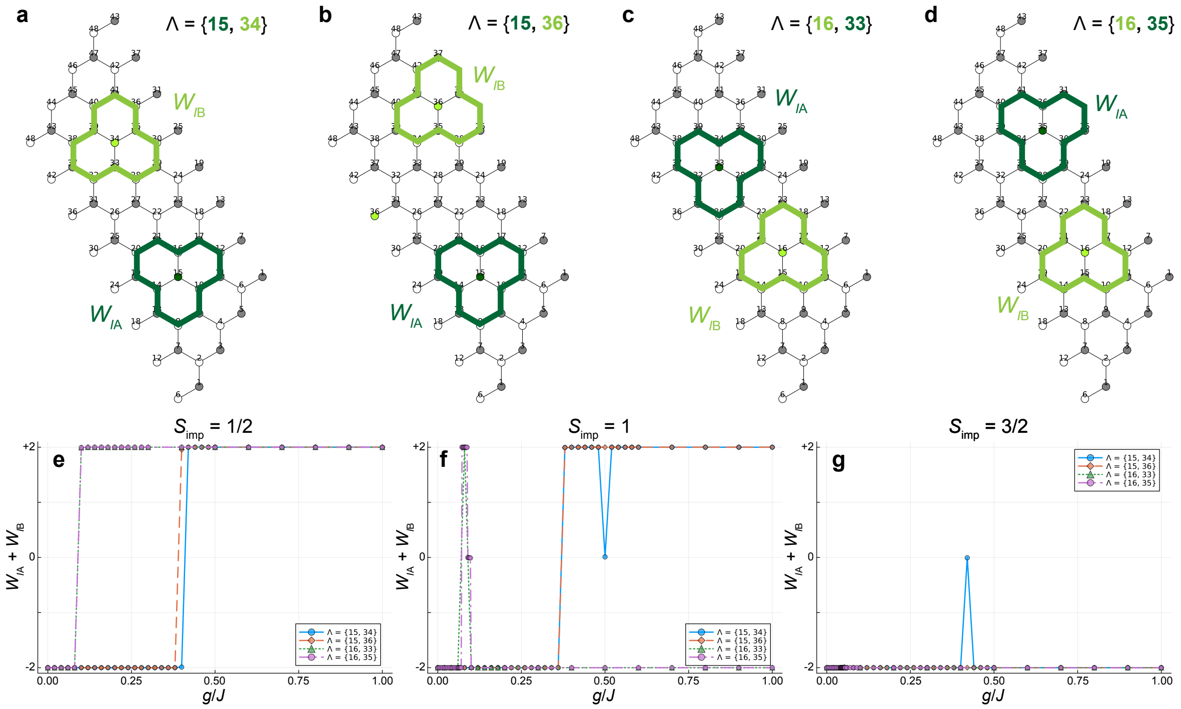


Supplementary Figure 4. 48-site clusters with two impurities are shown in **a** to **d**, as **a** $\Lambda = \{15, 34\}$, **b** $\Lambda = \{15, 36\}$, **c** $\Lambda = \{16, 33\}$, and **d** $\Lambda = \{16, 35\}$. Impurity-position dependence on flux-sector transition in **e** $S_{\text{imp}} = 1/2$, **f** $S_{\text{imp}} = 1$, and **g** $S_{\text{imp}} = 3/2$.

For the $S_{\text{imp}} = 1/2$ case, two-impurity results remain qualitatively the same compared to the single-impurity case, where the zero-flux sector is stabilized for large $g$ (see Supplementary Figure 4**e**). All four curves show a single bound-to-zero flux-sector transition, and the position of the impurities only affects the critical value of $g$.

For the $S_{\text{imp}} = 1$ case, more than one transition can happen in some of the configurations, and the ground-state flux sector for $g \gtrsim 0.4$ is highly dependent on the impurity position. This reinforces the idea that $S_{\text{imp}} = 1$ is the marginal case, which is discussed in the one-impurity results (see Supplementary note 3). In addition, at some particular values of $g$, we see $\sum_{\lambda=\text{A,B}} W_{I\lambda} = 0$, which implies $W_{IA} = -W_{IB}$. This "one-bound-flux sector" is recognized as a combination of the bound-flux and zero-flux sectors for the impurities. Note that multiple runs of DMRG confirm the presence of the one-bound-flux sector at these points consistently, implying that this is due to subtle energetic effects on the finite-size cluster instead of numerical errors.

Finally, for the $S_{\text{imp}} = 3/2$ case, we found that the zero-flux sector completely vanishes even at the intermediate coupling regime. Except for one point with the one-bound-flux sector, the general behavior is that the "two-bound-flux sector" dominates the phase diagram regardless of the impurity configuration. This suggests that multiple $S_{\text{imp}} = 3/2$ impurities can further stabilize bound flux on each impurity plaquette, making it a more promising system for identifying defect-induced fluxes compared to multiple quasivacancies [6].

## Supplementary Note 5: Comments on other clusters

We have confirmed, by using another type of finite-size clusters wrapped on a cylinder geometry as shown in Supplementary Figure 5, that our results summarized in Supplementary Table 1 and Supplementary Figure 4 remain quantitatively unchanged. That is, while the $S_{\text{imp}} = 3/2$ impurity tends to bind a $Z_2$ flux, the $S_{\text{imp}} = 1$ impurity suffers from severe position dependence.

When we switch the BCs of the cluster shown in Supplementary Figure 5, the system doesn't have the bound-flux sector at $g/J = 0$, which implies the strong finite-size effect in this system. Even in this system, however, $S_{\text{imp}} = 3/2$ impurities bind the $Z_2$ fluxes at $g/J \sim \mathcal{O}(1)$, resulting in the bound-flux sector in the strong-coupling limit.

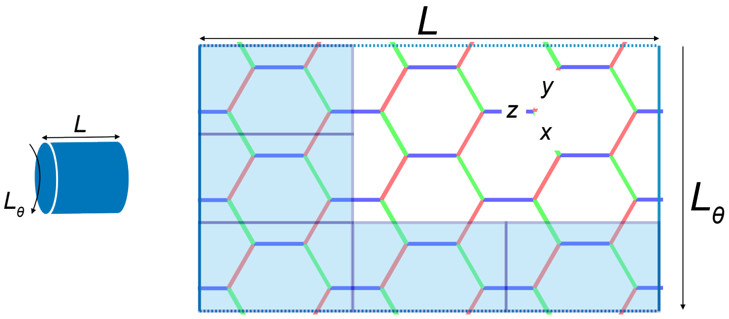


Supplementary Figure 5. The other cluster we have used to confirm the independence of cluster shape on the results in the main text.

## References

[1] Kitaev, A. Anyons in an exactly solved model and beyond. *Ann. of Phys.* **321**, 2 – 111 (2006).

[2] Feng, K., Perkins, N. B. & Burnell, F. J. Further insights into the thermodynamics of the kitaev honeycomb model. *Phys. Rev. B* **102**, 224402 (2020).

[3] Willans, A. J., Chalker, J. T. & Moessner, R. Disorder in a quantum spin liquid: Flux binding and local moment formation. *Phys. Rev. Lett.* **104**, 237203 (2010).

[4] Das, S. D., Dhochak, K. & Tripathi, V. Kondo route to spin inhomogeneities in the honeycomb kitaev model. *Phys. Rev. B* **94**, 024411 (2016).

[5] Vojta, M., Mitchell, A. K. & Zschocke, F. Kondo impurities in the kitaev spin liquid: Numerical renormalization group solution and gauge-flux-driven screening. *Phys. Rev. Lett.* **117**, 037202 (2016).

[6] Kao, W.-H., Knolle, J., Halász, G. B., Moessner, R. & Perkins, N. B. Vacancy-induced low-energy density of states in the kitaev spin liquid. *Phys. Rev. X* **11**, 011034 (2021).
